# Supplementary material for: A Novel Nonlinear Nonparametric Correlation Measurement With A Case Study on Surface Roughness in Finish Turning
Source: arXiv:2406.06924 source file (2024-06-11)
Supplement: Supplementary file 1 [file Appendix.tex]

\begin{tabular}{@{}ll@{}} 
\textbf{Symbol} & \textbf{Description} \\
$a\in A$ & \textbf{arc} (directed) from vertex $v_i$ to $v_j$, set of arcs \\
$\phantom{a\in{}}A^\text{p}_{v}$ & \quad arriving arcs into vertex $v$ (\emph{predecessor}) \\
$\phantom{a\in{}}A^\text{s}_{v}$ & \quad leaving arcs from vertex $v$ (\emph{successor}) \\[3pt]
$b \in B_{e}$ & \textbf{building}, set of buildings along edge $e$ \\
$b_\text{eff}$ & concurrence effect (parameter) \\[3pt]
$c\in C$ & \textbf{commodity}, set of commodities \\[3pt]
$e\in E$ & \textbf{edge}, set of edges \\[3pt]
& \dots \\[3pt]
$v\in V$ & \textbf{vertex}, set of vertices
\end{tabular}
